# Supplementary material for: Fast Training of Diffusion Transformer with Extreme Masking for 3D Point Clouds Generation
Source: arXiv:2312.07231 source file (2023-12-12)
Supplement: Supplementary file 1 [file vis_demo.tex]

\begin{figure*}[h!]
\vspace{-5mm}
\begin{center}
	\animategraphics[width=0.999\textwidth, loop, autoplay, final, nomouse, method=widget]{5}{./figs/teaser_m2bev/}{00002}{00017}	
	\vspace{-5mm}
	\caption{
	\footnotesize Qualitative results of FastDiT-3D, \todo{} \emph{The figure contains a short video clip best viewed by Adobe Reader.}
 	}%
	\label{fig:vis_demo}
\end{center}
\vspace{-10pt}
\end{figure*}
